# Supplementary material for: Reverberation: Learning the Latencies Before Forecasting Trajectories
Source: arXiv:2511.11164 source file (2026-10-19)
Supplement: Supplementary file 5 [file s2t1_efficiency.tex]

%%%%%%%%%%%%%%%%%%%%%%%
%% Author: Conghao Wong
%% Date: 2025-05-26 21:12:14
%% LastEditors: Ziqian Zou
%% LastEditTime: 2025-11-27 19:06:03
%% Github: https://cocoon2wong.github.io
%% Copyright 2025 Conghao Wong, All Rights Reserved.
%%%%%%%%%%%%%%%%%%%%%%%

\documentclass[../../paper.tex]{subfiles}

\begin{document}

\begin{table}[tbp]
    \caption{
        Inference Times and Memory Usages of \MODELSHORT~Models ($t_h = 8$, $t_f = 12$, forecasting 20 trajectories for each ego, on Apple M1 Mac mini).
    }
    \label{tab_efficiency}
    \centering
    \begin{tabular}{lcccccccc}
        \toprule
        Model & Parameters &
        \makecell{ADE/FDE\\(zara1)} &
        \makecell{Batch\\Size} &
        \makecell{Time\\(ms)} &
        \makecell{Memory\\(MB)} \\

        \midrule
        \multirow{3}{*}{\MODELSHORT} &
        \multirow{3}{*}{3,156,220} &
        \multirow{3}{*}{0.172/0.283}
        & 1         & 30    & 37.14 \\
        % &&& 20   & 35 & 45.96 \\
        % &&& 50   & 42 & 75.71 \\
        &&& 100     & 47    & 115.09 \\
        &&& 1000    & 190   & 535.30 \\

        \midrule
        \multirow{3}{*}{\MODELSHORT-a6} &
        \multirow{3}{*}{\makecell{1,216,670\\(w/o $\Delta \hatbf{Y}^i_\NON$)}} &
        \multirow{3}{*}{0.174/0.294}
        & 1         & \C{17}    & \CC{10.08} \\
        &&& 100     & 31        & 78.03 \\
        &&& 1000    & 159       & 395.99 \\

        \midrule
        \multirow{3}{*}{\MODELSHORT-a7} &
        \multirow{3}{*}{\makecell{2,079,710\\(w/o $\Delta \hatbf{Y}^i_\SOC$)}} &
        \multirow{3}{*}{0.176/0.297}
        & 1         & \CC{15}   & \C{16.21} \\
        &&& 100     & 22        & 26.29 \\
        &&& 1000    & 45        & 116.70 \\
        
        \bottomrule
    \end{tabular}
\end{table}

\end{document}
