# Supplementary material for: Reverberation: Learning the Latencies Before Forecasting Trajectories
Source: arXiv:2511.11164 source file (2026-10-19)
Supplement: Supplementary file 10 [file s4t1_meanstd_zara1.tex]

%%%%%%%%%%%%%%%%%%%%%%%
%% Author: Conghao Wong
%% Date: 2025-09-26 11:17:59
%% LastEditors: Conghao Wong
%% LastEditTime: 2025-09-26 17:13:52
%% Github: https://cocoon2wong.github.io
%% Copyright 2025 Conghao Wong, All Rights Reserved.
%%%%%%%%%%%%%%%%%%%%%%%

\documentclass[../../paper.tex]{subfiles}

\begin{document}

\begin{table*}[tbp]
    \caption{
        Statistical verifications of \MODELSHORT~model on zara1.
        Results are reported with ``mean $\pm$ std'' computed from 10 model runs.
    }
    \label{tab_meanstd_zara1}
    \centering
    \begin{tabular}{lccccccccccc}
        \toprule
        $K$ & minADE$_K$ & meanADE$_K$ & stdADE$_K$ & minFDE$_K$ & meanFDE$_K$ & stdFDE$_K$ \\

        \midrule
        1   & 0.7287 $\pm$ 0.2243 & 0.7654 $\pm$ 0.1903 & -                   & 1.6113 $\pm$ 0.5291 & 1.6768 $\pm$ 0.4327 & -                   \\
        2   & 0.5354 $\pm$ 0.1020 & 0.7541 $\pm$ 0.0826 & 0.3704 $\pm$ 0.0428 & 1.1541 $\pm$ 0.2369 & 1.6528 $\pm$ 0.2004 & 0.8522 $\pm$ 0.1152 \\
        4   & 0.3678 $\pm$ 0.0483 & 0.7977 $\pm$ 0.0341 & 0.4395 $\pm$ 0.0475 & 0.7587 $\pm$ 0.1081 & 1.7557 $\pm$ 0.0771 & 1.0262 $\pm$ 0.1230 \\
        8   & 0.2724 $\pm$ 0.0137 & 0.7666 $\pm$ 0.0288 & 0.4338 $\pm$ 0.0354 & 0.5330 $\pm$ 0.0264 & 1.6807 $\pm$ 0.0678 & 1.0086 $\pm$ 0.0850 \\
        12  & 0.2145 $\pm$ 0.0036 & 0.7331 $\pm$ 0.0279 & 0.4201 $\pm$ 0.0173 & 0.3934 $\pm$ 0.0090 & 1.6067 $\pm$ 0.0649 & 0.9764 $\pm$ 0.0420 \\
        16  & 0.1924 $\pm$ 0.0021 & 0.7577 $\pm$ 0.0089 & 0.4398 $\pm$ 0.0048 & 0.3343 $\pm$ 0.0061 & 1.6628 $\pm$ 0.0195 & 1.0228 $\pm$ 0.0101 \\
        20  & 0.1730 $\pm$ 0.0002 & 0.7482 $\pm$ 0.0002 & 0.4348 $\pm$ 0.0001 & 0.2836 $\pm$ 0.0009 & 1.6413 $\pm$ 0.0005 & 1.0122 $\pm$ 0.0005 \\
        40  & 0.1682 $\pm$ 0.0001 & 0.7481 $\pm$ 0.0001 & 0.4292 $\pm$ 0.0001 & 0.2693 $\pm$ 0.0006 & 1.6414 $\pm$ 0.0001 & 0.9993 $\pm$ 0.0002 \\
        60  & 0.1656 $\pm$ 0.0001 & 0.7481 $\pm$ 0.0001 & 0.4275 $\pm$ 0.0001 & 0.2620 $\pm$ 0.0001 & 1.6414 $\pm$ 0.0001 & 0.9952 $\pm$ 0.0001 \\
        100 & 0.1630 $\pm$ 0.0001 & 0.7481 $\pm$ 0.0000 & 0.4260 $\pm$ 0.0001 & 0.2544 $\pm$ 0.0003 & 1.6415 $\pm$ 0.0001 & 0.9918 $\pm$ 0.0001 \\
        \bottomrule
    \end{tabular}
\end{table*}

\end{document}
