# Supplementary material for: Reverberation: Learning the Latencies Before Forecasting Trajectories
Source: arXiv:2511.11164 source file (2026-10-19)
Supplement: Supplementary file 14 [file s6_latencies.tex]

%%%%%%%%%%%%%%%%%%%%%%%
%% Author: Conghao Wong
%% Date: 2025-11-25 15:45:16
%% LastEditors: Conghao Wong
%% LastEditTime: 2025-11-28 10:57:59
%% Github: https://cocoon2wong.github.io
%% Copyright 2025 Conghao Wong, All Rights Reserved.
%%%%%%%%%%%%%%%%%%%%%%%

\documentclass[../../paper.tex]{subfiles}

\begin{document}

\section{Discussions of Latencies, Dependencies, Temporal Attention, and Temporal Convolution}

Learning and forecasting the temporal latencies of agents for handling trajectory-changing events is the main concern of this manuscript.
This section provides clear formula descriptions of several relevant conceptions, explaining why the (temporal) latencies are significant to this task, and why current temporal dependencies, temporal attention, and temporal convolution approaches cannot address the modeling of latencies.

\subsection{Temporal Dependencies and Latencies}

Temporal dependency characterizes how strongly one moment (either an observation or a prediction moment) contributes to another.
Formally, most dependency-based models aim to estimate a mapping of the form
\begin{equation}
    \mathcal{D}(t_1, t_2) = g \left(
        \mathbf{f}(t_1), \mathbf{f}(t_2)
    \right),
\end{equation}
where $g$ measures temporal correlation between representations (or embeddings) $\mathbf{f}(t_1)$ and $\mathbf{f}(t_2)$ of two considered temporal steps $t_1$ and $t_2$.

In recurrent-networks-based methods, these dependencies are mostly considered as the relationship of two adjacent temporal steps, like a $t_1 = t$ and the other $t_2 = t + 1$, thus learning how to build recurrent cells within RNNs or LSTMs to infer features of the next step based on the current status (or saved memories if available).
For models using the Transformer, such dependencies have become less recurrent and more relative to the global.
These methods extract features over the observation time period (temporal attention is not discussed here, see the next section) and holistically evaluate how these features contribute to the prediction time period.
Thus, temporal dependencies focus more on how different moments affect or contribute to each other.

Differently, temporal latency concerns more about when an event at time $t_0$ becomes behaviorally effective, or starts to change the outcome of the system.
It describes a temporal shift
\begin{equation}
    \label{eq_latency_shift}
    \mathcal{D}: t_0 \to t_0 + \Delta t_0
\end{equation}
indicating the onset of its impact, and further the offset, \IE, the whole life-cycle of this event.
Thus, latencies represent the concept of a time latency rather than a simple intensity contribution, with a focus on considering how the impact of an event changes over the timeline.
In short, dependencies operate in the magnitude domain, whereas latencies operate in the time-index domain.
In human-agent reasoning, this corresponds to the distinction between what matters (dependencies) and when it starts to matter (latencies).
This is the main difference between temporal dependencies and latencies.

\subsection{Why Temporal Attention Does Not Explicitly Encode Latencies}

Intuitively, attention is able to localize a moment in a time series or a representation on that moment that contributes most to the classification result or to the future.
In detail, for a specific temporal moment $t = t_0$, its attention is computed as
\begin{equation}
    a_{t_0} = \sum_\tau g(t_0, \tau) \mathbf{f}(\tau),
\end{equation}
where $g$ simply represents the softmax operation of features.
Here, all historical moments are considered immediately accessible to each other moment through soft alignment.

In other words, attention treats influence as continuous and instantaneous, meaning that it does not include and specify that the impact of any event should begin at a later step or should finish at a further future, thus does not simulate or explicitly model the structured shift of latencies defined in \EQUA{eq_latency_shift}.
Temporal attention is permutation-sensitive but not temporally directional.
That is, attention explains how much a moment is relevant or is important, not when its influence begins or ends across time.

\subsection{Why Temporal Convolution Does Not Explicitly Encode Latencies}

Since having the form of matrix multiplication, the proposed reverberation transform has some similarity with temporal convolution.
However, it should be noted that reverberation transform is not a convolution or a variant of convolution, and in turn convolution does not explicitly model representations of latencies.
Formally, temporal convolution applies a fixed kernel $h(t)$ across time to obtain the outcome:
\begin{equation}
    \mathbf{y}(t) = \sum_{\delta} h(\delta) \mathbf{x}(t - \delta).
\end{equation}

This formulation captures local smoothness or short-term patterns, but all events are filtered with the same kernel $h$, leading to the same temporal pattern.
Also, convolution cannot model event-specific or state-dependent latencies, since the temporal-static kernel $h$ cannot distinguish an event or a temporal step should influence the outcome at a specific future moment.
In other words, convolution also modifies magnitude, not time indices.
It smooths or sharpens signals but does not implement temporal rescheduling, thus it still does not explicitly model temporal latencies.

On the contrary, the proposed reverberation transform differs significantly from attention and convolution.
Given similarities $\mathbf{F}$, the transform $\overline{\mathbf{F}} = \mathbf{G}^\top \mathbf{F} \mathbf{G}$ operates directly on the time indices.
Here, the kernel $\mathbf{R}$ maps each historical event (could be represented as a historical step or a social partition) to exactly where in the future it will be reconsidered, thus acting as a learnable temporal scheduling function.
Meanwhile, the other kernel $\mathbf{G}$ mixes multiple latency hypotheses, enabling diverse latency-aware futures.
Together, they create a \emph{temporal re-indexing} operator:
\begin{equation}
    \mathcal{R}: t_o \to t_o + \Delta t_0.
\end{equation}
Different from amplifying or filtering temporal correlation, the reverberation transform relocates historical influence onto future steps, yielding structured, physically interpretable latencies before forecasting trajectories.

\end{document}
